# Supplementary material for: M\"obius Convolutions for Spherical CNNs
Source: arXiv:2201.12212 source file (2022-05-12)
Supplement: Supplementary file 1 [file supp_main.tex]

\section{Integration and Differentiation}
\label{a:intdiff}
\input{supp/supp_intdiff}

\section{Equivariance of \mob{} Convolutions}
\label{a:equivariance}
\input{supp/supp_equiv}

\section{Transformation of Functions}
\label{a:filter_xform}
\input{supp/supp_xform}

\section{Memory Footprint and Run Time}
\label{a:overhead}
\input{supp/supp_overhead}

\section{Segmentation}
\label{a:seg}
\input{supp/supp_seg}
